# Supplementary material for: Evaluating Copyright Takedown Methods for Language Models
Source: arXiv:2406.18664 source file (2024-10-11)
Supplement: Supplementary file 1 [file appendix.tex]

% \appendix
% \newpage

% \subsection{Methods details}
% \label{app:method_detail}
